# Supplementary material for: RoPAWS: Robust Semi-supervised Representation Learning from Uncurated Data
Source: arXiv:2302.14483 source file (2023-02-28)
Supplement: Supplementary file 1 [file cifar.tex]

\section{Additional CIFAR-10 results}
\label{appx:cifar}

Table~\ref{tab:cifar-more} provides additional CIFAR-10 results using 4 labels for each class. RoPAWS gives a consistent gain over PAWS. However, the original PAWS is more prone to confirmation bias in this setup, and RoPAWS is slightly worse than the prior arts; PAWS needs a sufficient number of labels to model densities via KDE.

\begin{table}[h]
\centering\small
\caption{
Test accuracy (\%) of semi-supervised learning methods trained on CIFAR-10 (4 labels per class) and extra unlabeled data denoted by (+ extra), using (a) no extra and (b) CIFAR-100. 
}\label{tab:cifar-more}
\begin{tabular}{lll}
\toprule
& CIFAR-10 & CIFAR-10 (+ CIFAR-100) \\
\midrule
FixMatch
& 86.2\stdv{3.4} \phantom{\up{3.0}}
& 67.4 \blkstdv \phantom{\up{11.6}} \\
\midrule
PAWS
& 85.7\stdv{2.4} \phantom{\up{3.0}}
& 50.3\stdv{2.2} \phantom{\up{11.6}} \\
\sname (ours)
& 88.7\stdv{2.2} \up{3.0}
& 63.5\stdv{4.3} \up{13.2} \\
\bottomrule
\end{tabular}
\end{table}
