# Supplementary material for: RoPAWS: Robust Semi-supervised Representation Learning from Uncurated Data
Source: arXiv:2302.14483 source file (2023-02-28)
Supplement: Supplementary file 2 [file imagenet.tex]

\section{Additional ImageNet results}
\label{appx:imagenet}

\tbd{Add more imagenet results!}

\begin{table}[h]
\centering\small
\caption{
Test accuracy (\%) of RoPAWS on ImageNet using Soft-NN or Fine-tuned classifier.
% Subscripts denote the gain over PAWS. RoPAWS achieves the state-of-the-art.
}\label{tab:imagenet-more}
\begin{tabular}{lcccc}
\toprule
& \multicolumn{2}{c}{Label 1\%} & \multicolumn{2}{c}{Label 10\%} \\
\cmidrule(lr){2-3}\cmidrule(lr){4-5}
& Soft-NN & Fine-tune & Soft-NN & Fine-tune \\
\midrule
PAWS          & 64.2 & 66.5 & 73.1 & 75.5 % 75.9 & 79.2
\\
\sname (ours) & 64.4 & 
\\
\bottomrule
\end{tabular}
%
% \begin{tabular}{llcccccc}
% \toprule
% & & \multicolumn{3}{c}{IN-1k (no extra)} & \multicolumn{3}{c}{IN-1k (+ IN-21k)} \\
% \cmidrule(lr){3-5}\cmidrule(lr){6-8}
% & & 1\% & 10\% & 100\% & 1\% & 10\% & 100\% \\
% \midrule
% \multirow{2}{*}{PAWS}
% & Soft-NN
% & 64.2 & 73.1 & 75.9
% \\
% & Fine-tune
% & 66.5 & 75.5 & 79.2
% \\
% \midrule
% \multirow{2}{*}{\sname (ours)}
% & Soft-NN
% \\
% & Fine-tune
% \\
% \bottomrule
% \end{tabular}
%
\end{table}
